# Supplementary material for: Cross Project Software Vulnerability Detection via Domain Adaptation and Max-Margin Principle
Source: arXiv:2209.10406 source file (2022-09-19)
Supplement: Supplementary file 2 [file supp_ved.tex]

In this section, we summarize the information of datasets used in
our experiments, the required packages and the instructions for reproducing
the experimental results of our proposed DAM2P method.

\subsection{Setup}

\paragraph{Datasets}

We used the real-world datasets experimented in \citet{vannguyen2019dan,van-nguyen-dual-dan-2020}.
These contain the source code of vulnerable functions (vul-funcs)
and non-vulnerable functions (non-vul-funcs) obtained from six real-world
software project datasets, namely FFmpeg (\#vul-funcs: 187 and \#non-vul-funcs:
5427), LibTIFF (\#vul-funcs: 81 and \#non-vul-funcs: 695), LibPNG
(\#vul-funcs: 43 and \#non-vul-funcs: 551), VLC (\#vul-funcs: 25 and
\#non-vul-funcs: 5548), and Pidgin (\#vul-funcs: 42 and \#non-vul-funcs:
8268). These datasets cover multimedia and image application categories.

In the experiments, to demonstrate the capability of our proposed
method in the transfer learning for cross-domain software vulnerability detection
(SVD) (i.e., transferring the learning of software vulnerabilities
(SVs) from labelled projects to unlabelled projects belonging to different
application domains), the datasets (FFmpeg, VLC, and Pidgin) from
the multimedia application domains were used as the source domains,
whilst the datasets (LibPNG and LibTIFF) from the image application
domains were used as the target domains. It is worth noting that in
the training process we hide the labels of datasets from the target
domains. We only use these labels in the testing phase to evaluate
the models\textquoteright{} performance. Moreover, we used 80\% of
the target domain without labels in the training process, while the
rest 20\% was used for evaluating the domain adaptation performance.
We note that these partitions were split randomly as used in the baselines.

\paragraph{Requirements}

We implemented our DAM2P method and baselines using Tensorflow \citep{abadi2016tensorflow}
(version 1.15) and Python (version 3.6). Other required packages are scikit-learn and numpy.

\subsection{Running source code samples}

Here, we provide the instructions for using the source code samples
of our DAM2P method the on the pair of the source domain (FFmpeg) to the target domain (LibPNG).

For our method and baselines, after training the model on the training set, we can find out the best model (i.e., based on the results of AUC, Recall, Precision and F1-measure on the validation set) which then will be used to obtain the best results on the testing set.

In our source code samples, for the demonstration purpose, we design to train the model using the training set, evaluate the model performance on the testing set after every specific iteration, and save the high results (in a list) on the testing set corresponding to the used hyper-parameters.

\paragraph{Folders and files}
\begin{itemize}
\item The folder named ``datasets'' consists of all of the necessary
files containing the source domain (FFmpeg) and target domain (LibPNG) data.
\item The file named ``DAM2P\_train\_evaluate.py'' is the source code of our proposed DAM2P method used for the training and evaluating
processes.
\item The file named ``Utils.py'' is a collection of supported Python functions used in the training and evaluating
processes of the model.
\end{itemize}

\textbf{Note that}: Please download
the dataset and the source code files via this link \href{https://drive.google.com/drive/folders/1Rlabx8LSBdTGM5CyW39KNX6Yc9vcS081?usp=sharing}{https://drive.google.com/drive/folders/1R.}

\paragraph{The model configuration}

For the DAM2P model configuration, please read \emph{the Model configuration
section} in the supplementary material for details.
